# Supplementary material for: Local Occupancy-Enhanced Object Grasping with Multiple Triplanar Projection
Source: arXiv:2407.15771 source file (2024-07-22)
Supplement: Supplementary file 1 [file X_suppl.tex]

\clearpage
\setcounter{page}{1}

\appendix

\section{Implementation Details}
\textbf{Model architecture}. Here we provide more details of our model. The 14-layer 3-D UNet backbone initiates by voxelizing the input point cloud (with a voxel size of 5mm) and then encodes the point cloud through convolution/deconvolution modules. The voxel resolution undergoes a down-sampling of (2, 4, 8, 16) times and subsequently up-sampled to restore the original resolution within the UNet framework. Consequently, each point in the point cloud is embedded with $C_P=256$ dimensions based on the corresponding voxel. Following the approach proposed by~\cite{Wang2021GraspnessDI}, the grasp affordance segmentation and the view-wise affordance regression are calculated by two 2-layer MLPs separately. Points with a grasp affordance greater than 0.5 are identified as the affordance area. The view-wise affordance, representing grasp quality across 300 discrete grasp directions, is exclusively calculated for the sampled grasp points. In the generation of multi-group tri-plane rotations, we define $\vq_1$ as the identity rotation and $\vq_2$ as orthometric to $\vq_1$ to maximize the rotation distance. Specifically, we set $\vq_1=(1, 0, 0, 0)$ and $\vq_2=(0, \frac{1}{\sqrt{3}}, \frac{1}{\sqrt{3}}, \frac{1}{\sqrt{3}})$. During the aggregation of point cloud embeddings and point density through triplanar projection, we normalize the coordinates of the point cloud to the range $[0, 1]$ along each axis. In the local occupancy query stage, the encoders $\Tilde{\mathcal{E}}_1, \Tilde{\mathcal{E}}_2, \mathcal{E}_{PE}$, and the decoder predicting occupancy probability, are all 2-layer MLPs.

For the local shape feature extraction and grasp pose estimation in each local grasp region, an illustration is shown in~\cref{fig:image9}. Concretely, 32 key points are sampled from $\mP_o$, and their corresponding queried features undergo processing with max-pooling to form a holistic feature. Meanwhile, the 4 point set abstraction layers in the explicit shape encoder sample (32, 8, 4, 1) points respectively, ultimately outputting the shape feature with 512 dimensions.  Finally, these two features are concatenated and the grasp scores and grasp widths are predicted for 12 possible in-plane rotations combined with 4 possible depths. The 12 in-plane rotations span from 0 to 180 degrees at 15-degree intervals, while the 4 possible depths range from 1cm to 4cm with a 1cm interval.

\textbf{Real-world experiment}.
In our real-world experiment, illustrated in~\cref{tab:realexp setting}, the process unfolds as follows: the camera initially captures a depth image of the grasping scene, which is subsequently transformed into a point cloud using the camera intrinsics. Upon our model proposing several grasp poses, the grasp pose with the highest grasp score is selected and then transformed from the camera frame to the robotic arm frame based on the hand-eye calibration. Then the grasp is executed and success is determined if the object does not fall throughout the gripper's movement to the target location. In the event of a failed grasp, the object is repositioned until all objects are successfully grasped. For our experiment, we curated a selection of 42 objects, encompassing fruit models, 3-D printed objects (such as cameras and bottles), and common daily items (including boxes, mice, and toys). Each grasp scene consists of 5-8 objects, culminating in a total of 50 target objects for the experiment. The grasping video is available in the supplementary material file.

\begin{figure*}[ht]
\begin{center}
\includegraphics[width=\linewidth]{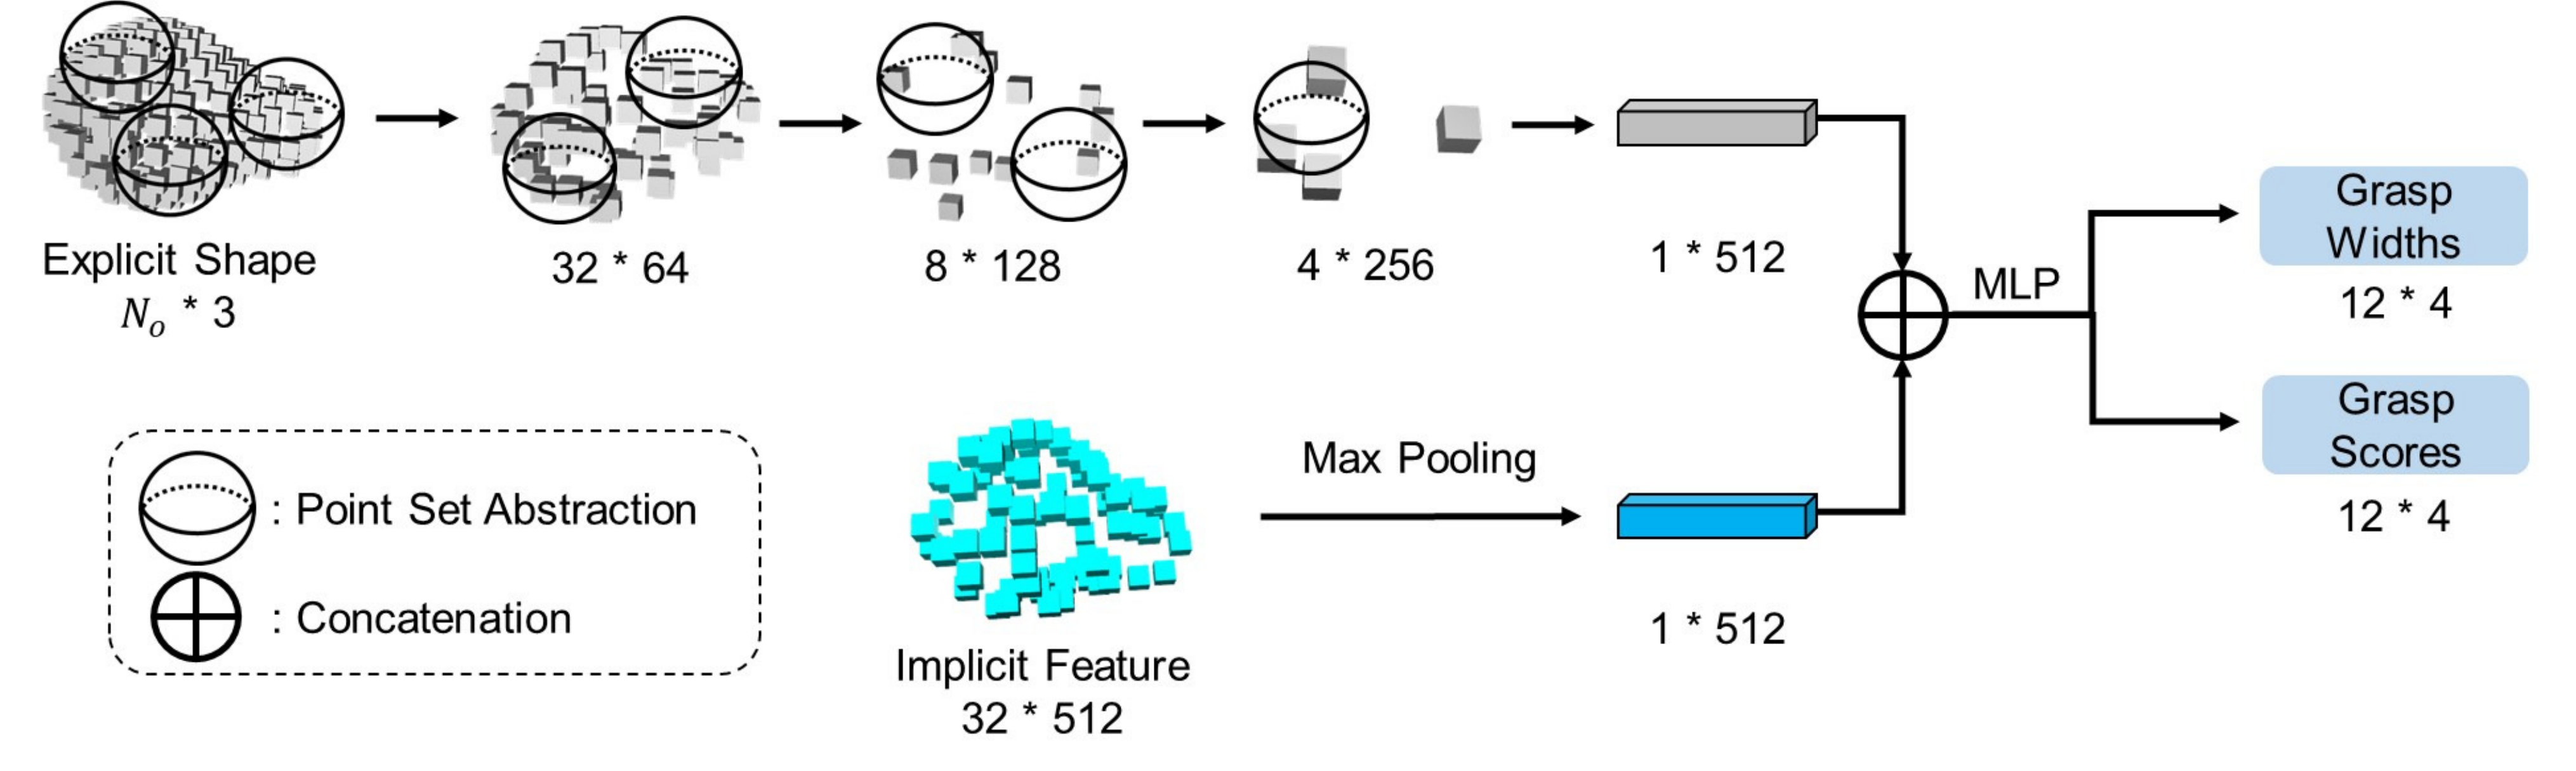}
\end{center}
   \caption{\small The architecture of  the local shape feature extraction and grasp pose estimation stage.}
\label{fig:image9}
\end{figure*}

\begin{table}
    \caption{\footnotesize The number of objects and volumetric IOU of different shape levels within the grasp regions.}
  \centering  
  \begin{footnotesize}
  \begin{tabular}{c|cc|ccc}
    \toprule
    \multirow{2}{*}{\bf Level} & \multicolumn{2}{c|}{\bf Number}          & \multicolumn{3}{c}{\bf IOU}                                          \\ \cline{2-6} 
                       & \multicolumn{1}{c|}{Train} & Test & \multicolumn{1}{c|}{Seen} & \multicolumn{1}{c|}{Similar} & Novel \\ \hline
    Easy                   &    12   &  17  &    0.763    &  0.740   & 0.709      \\
    Middle                 &     23   &  32  &    0.715   &  0.676  &  0.622     \\
    Hard                   &    5  &   26 &    0.572   &    0.541   &  0.465     \\ 
    \bottomrule
  \end{tabular}
  \end{footnotesize}

\label{tab:shape ablation}
\end{table}

\section{More Experiments}
To further study how well our occupancy prediction method generalizes to different types of shapes and how much the number of training objects affects the generalization ability, we compare the number of objects and the volumetric IOU within the grasp regions on different shape complexity levels in ~\cref{tab:shape ablation}. Specifically, we manually divide the objects in GraspNet-1Billion~\cite{graspnet1b} into three complexity levels. The \emph{easy} level mainly contains boxes and fruit with simple shapes. The \emph{middle} level includes ordinary tools and vessels, such as bottles, bowls and drills. The \emph{hard} level contains some 3D-printed models and animal models with complicated shapes. To calculate the volumetric IOU of each object in the scene, we assign each occupied voxel to the nearest object according to the segmentation label. The result shows that our method generalizes better to regular shapes (e.g. ball, cuboid, cylinder and their variants). However, the performance on \emph{hard} level is notably lower than the other levels, indicating higher shape complexity and fewer training data still challenge the ability of generalizing to novel complex shapes.

\section{Visualization}
For better visualization, we recommend readers to see the GIF visualizing results in the supplementary material file. Examples of predicted local occupancy and grasp poses compared with the GSNet~\cite{Wang2021GraspnessDI} baseline are shown in ~\cref{fig:vis1,fig:vis2}.  It can be seen that the baseline method generates some high-scoring grasp poses with risk of collision, indicating these local shape features wrongly learns the complete shape without occupancy enhancement. To the contrary, local occupancy prediction is able to complete the objects in most of the grasping-related regions, providing essential shape information for accurate grasp pose estimation. Therefore, our method alleviates the risk of collision with the objects and proposes more reasonable grasp poses. 

\section{Limitations}
As mentioned in the main text, the local occupancy prediction is exclusively supervised within the grasp affordance areas. Consequently, when the grasp affordance segmentation fails in some challenging scenes (e.g., severely rugged objects), the occupancy prediction module may encounter a generalization problem on these shapes due to the lack of such training examples. This could lead to incorrect occupancy prediction, adversely affecting grasp pose estimation. We think that such limitation could be mitigated by a more balanced grasp point sampling during training, encompassing both within and outside the affordance areas, thereby improving generalization across diverse shapes.

\begin{figure*}[h]
\begin{center}
\includegraphics[width=\linewidth]{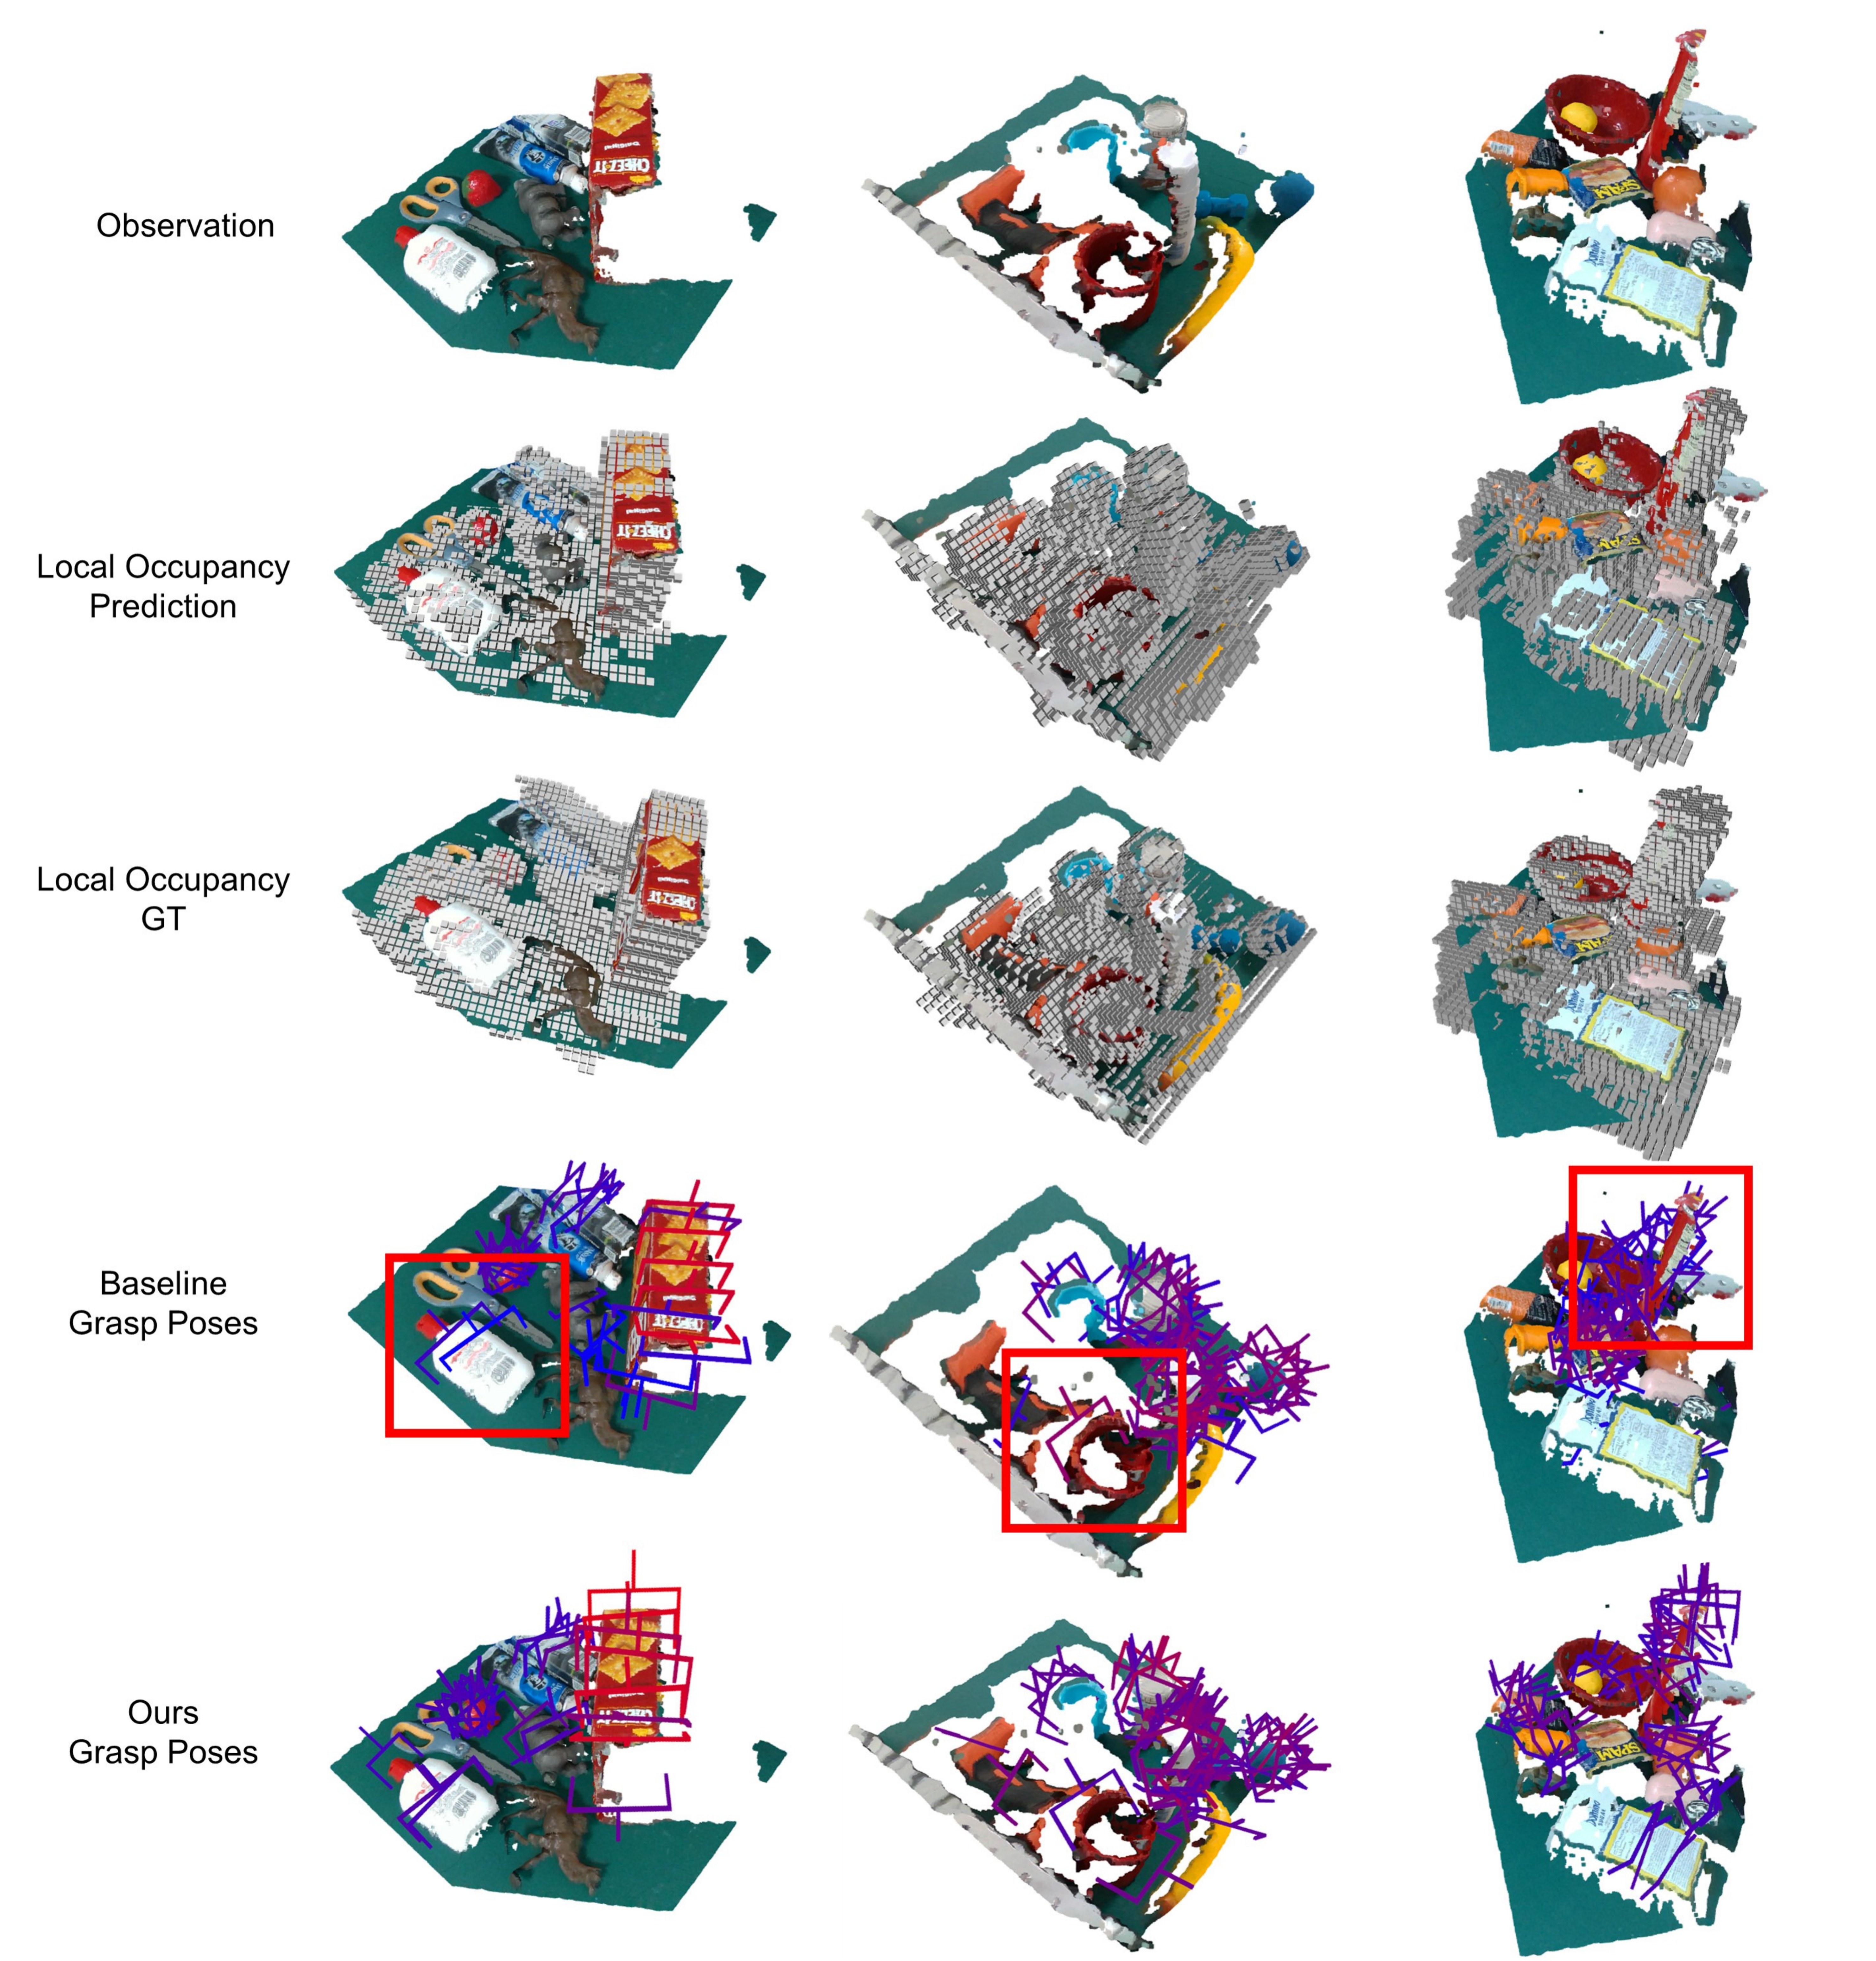}
\end{center}
   \caption{\small Visualizations of predicted local occupancy and grasp poses. Bad grasp poses proposed by the baseline are marked with \textcolor{red}{red} boxes.}
\label{fig:vis1}
%\vspace{-0.1in}
\end{figure*}

\begin{figure*}[h]
\begin{center}
\includegraphics[width=\linewidth]{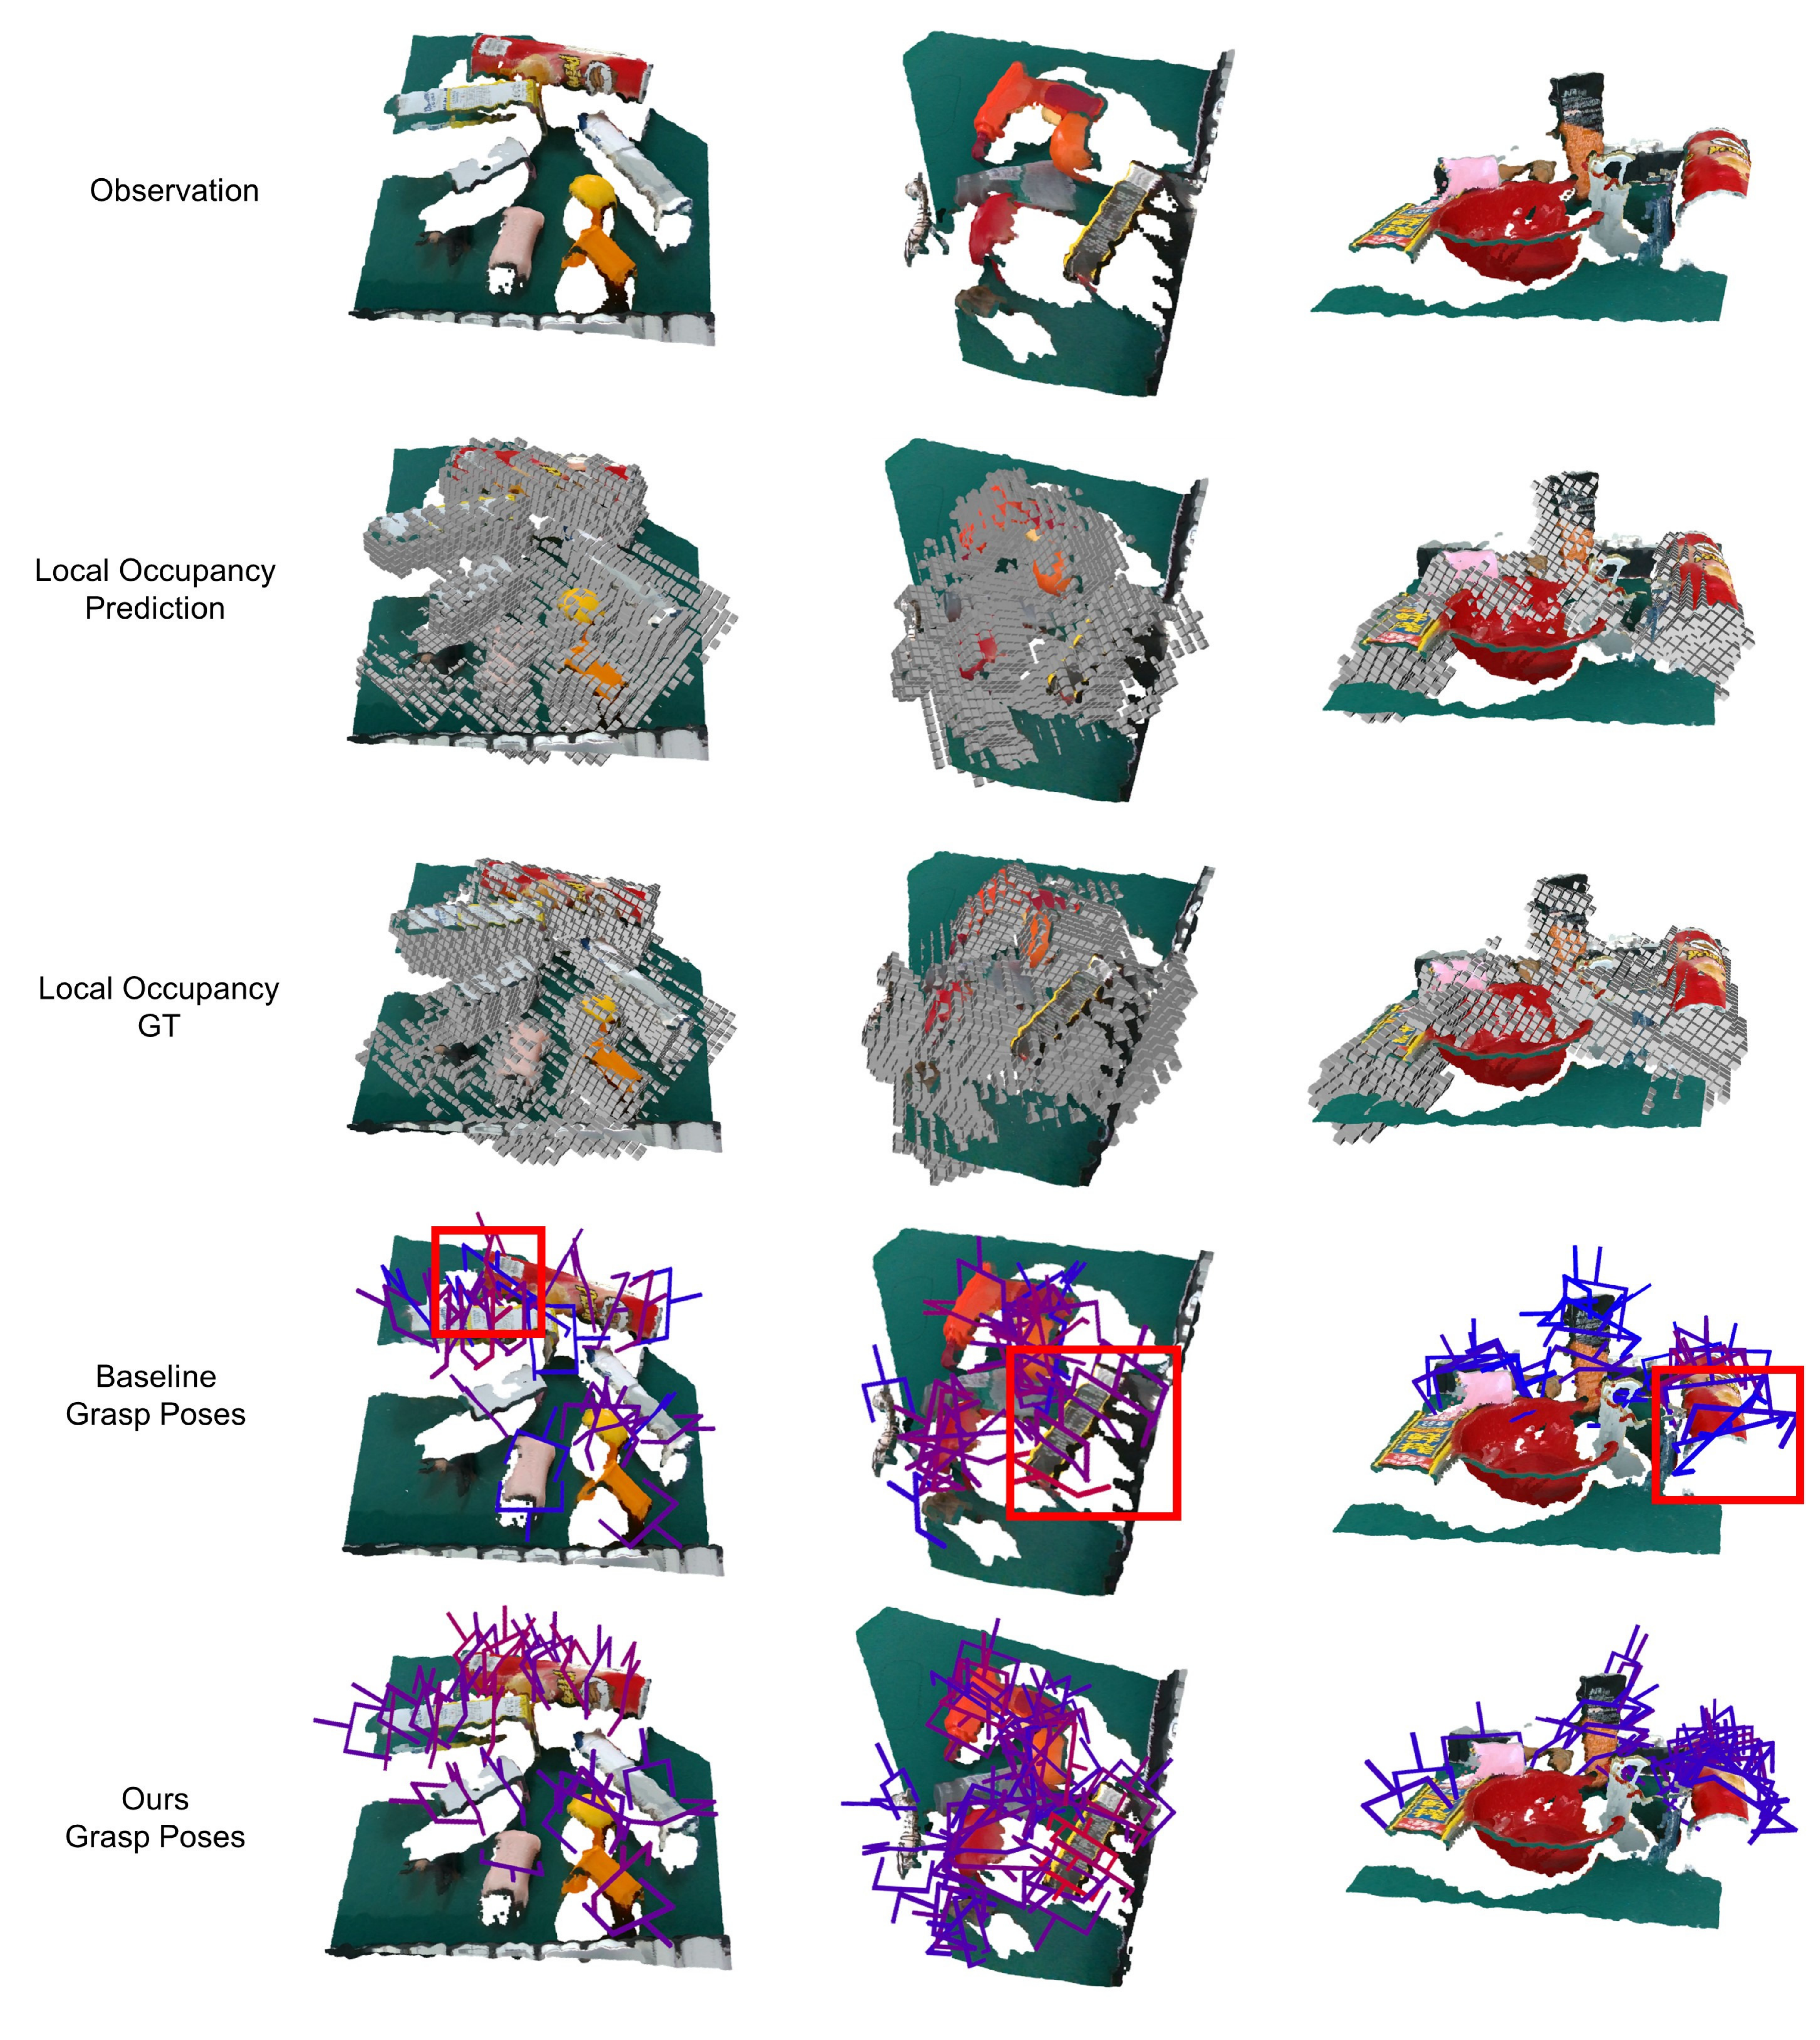}
\end{center}
   \caption{\small Visualizations of predicted local occupancy and grasp poses.Bad grasp poses proposed by the baseline are marked with \textcolor{red}{red} boxes.}
\label{fig:vis2}
%\vspace{-0.1in}
\end{figure*}
